# Supplementary material for: Solid-solid phase equilibria in the NaCl-KCl system
Source: arXiv:2003.09745 ancillary file (2020-04-15)
Supplement: Supplementary file 1 [file supplementary_material.pdf]

# Supplementary Material: Solid–solid phase equilibria in the NaCl–KCl system

Jamshed Anwar,[1,a)] Christian Leitold,[2,3,a)] and Baron Peters[2,4]
[1)]Department of Chemistry, Lancaster University, Lancaster, LA1 4YW, United Kingdom
[2)]Department of Chemical and Biomolecular Engineering, University of Illinois at Urbana-Champaign, Urbana, IL 61801, USA
[3)]Faculty of Physics, University of Vienna, 1090 Wien, Austria (present affiliation)
[4)]Department of Chemistry, University of Illinois at Urbana-Champaign, Urbana, IL 61801, USA

(Dated: March 13, 2020)

## I. FREE ENERGY FROM THERMODYNAMIC INTEGRATION

We follow the approach outlined in work by Anwar, Frenkel, and Noro[1] to obtain the Helmholtz free energy of pure NaCl and KCl crystals. The basic idea is to smoothly transform a reference system with analytically known free energy into the actual system of interest by varying a coupling parameter $\lambda$. Here, the reference system is an Einstein crystal. The potential energy of the coupled system is given as

$$U_\lambda(\mathbf{r}^N) = \lambda U_R(\mathbf{r}^N) + (1-\lambda)U_E(\mathbf{r}^N), \tag{1}$$

where $U_R(\mathbf{r}^N)$ is the "real" potential energy of the system and $U_E(\mathbf{r}^N)$ is the potential energy of an Einstein crystal, i. e. a system of non-interacting harmonic oscillators. For technical reasons, it is important to perform the thermodynamic integration using an additional constraint of a fixed center of mass, so the final result for the free energy per molecule of the real system comprises of three terms:

$$\hat{F}_R = \hat{F}_{E(CM)} + \Delta\hat{F}_{E(CM)\to R(CM)} + \Delta\hat{F}_{R(CM)\to R}, \tag{2}$$

where the subscripts $R$, $E$, and $CM$ refer to the real crystal, the Einstein crystal, and fixed center of mass respectively. Of these three terms, the first and the third are known analytically. In the case of NaCl, for the first term we have

$$\begin{aligned}\frac{\hat{F}_{E(CM)}}{k_\mathrm{B}T} &= 3N_\mathrm{Na}\ln\Lambda_\mathrm{Na} + 3N_\mathrm{Cl}\ln\Lambda_\mathrm{Cl} - \frac{3N_\mathrm{Na}}{2N_\mathrm{NaCl}}\ln\left(\frac{2\pi}{\beta\gamma_\mathrm{Na}}\right)\\ &\quad - \frac{3N_\mathrm{Cl}}{2N_\mathrm{NaCl}}\ln\left(\frac{2\pi}{\beta\gamma_\mathrm{Cl}}\right) - \frac{3}{2N_\mathrm{NaCl}}\ln\left(\frac{\beta\gamma_\mathrm{Na}}{2\pi N_\mathrm{Na}\mu_\mathrm{Na}^2}\right)\\ &\quad - \frac{3}{2N_\mathrm{NaCl}}\ln\left(\frac{\beta\gamma_\mathrm{Cl}}{2\pi N_\mathrm{Cl}\mu_\mathrm{Cl}^2}\right)\\ &\quad - \frac{3}{2N_\mathrm{NaCl}}\ln\left(\frac{\beta h^2}{2\pi\,(N_\mathrm{Na}m_\mathrm{Na} + N_\mathrm{Cl}m_\mathrm{Cl})}\right),\end{aligned} \tag{3}$$

where $h$ is Planck's constant, $\mu_i = m_i/(N_\mathrm{Na}m_\mathrm{Na}+N_\mathrm{Cl}m_\mathrm{Cl})$ is the fractional mass of each ion, and $\gamma_i$ is the associated force constant in the Einstein crystal. Similarly, the third term is

$$\begin{aligned}\frac{\Delta\hat{F}_{\mathrm{NaCl}(CM)\to\mathrm{NaCl}}}{k_\mathrm{B}T} &= \frac{1}{N_\mathrm{NaCl}}\ln\left(\frac{N_\mathrm{NaCl}}{V}\right)\\ &\quad + \frac{3}{2N_\mathrm{NaCl}}\ln\left(\frac{\beta h^2}{2\pi\,(N_\mathrm{Na}m_\mathrm{Na} + N_\mathrm{Cl}m_\mathrm{Cl})}\right).\end{aligned} \tag{4}$$

The middle term is the one obtained from numerically integrating simulation results:

$$\Delta\hat{F}_{E(CM)\to\mathrm{NaCl}(CM)} = \frac{\beta}{N_\mathrm{NaCl}}\int_0^1 d\lambda\,\langle U_\mathrm{NaCl} - U_E\rangle_\lambda\,. \tag{5}$$

We perform this integral using Gauss–Legendre quadrature with $n = 16$ nodes. Results are presented in Tab. I. Note that the free energies presented in the main text use a thermal de Broglie wavelength of 1 Å for all species to enable easier comparison with published values of Aragones, Sanz, and Vega.[2]

| $T$ | $\hat{F}_\mathrm{NaCl}/k_\mathrm{B}T$ | $\hat{F}_\mathrm{KCl}/k_\mathrm{B}T$ |
|---|---|---|
| 298 | $-316.512 \pm 0.005$ | $-289.903 \pm 0.004$ |
| 600 | $-162.853 \pm 0.005$ | $-150.357 \pm 0.005$ |

Table I. Helmholtz free energies for pure crystalline phases of NaCl and KCl from thermodynamic integration using the true thermal de Broglie wavelength for both molecules. In analogy to $\hat{G}$, $\hat{F}$ denotes the Helmholtz free energy per ion pair.

## II. FORCE FIELD COMPARISON

In Fig. 1, we show the effect of the slight change of the $B$, $C$, and $D$ parameters for the Cl–Cl interaction when compared to work by Aragones, Sanz, and Vega.[2]

## III. LATTICE PARAMETERS OF THE MIXTURE

Inspired by Vegard's law, we have fitted the lattice constant with a linear function of composition and temperature,

$$a \approx c_x x + c_T T + a_0. \tag{6}$$

[a)]J. Anwar and C. Leitold contributed equally to this work.

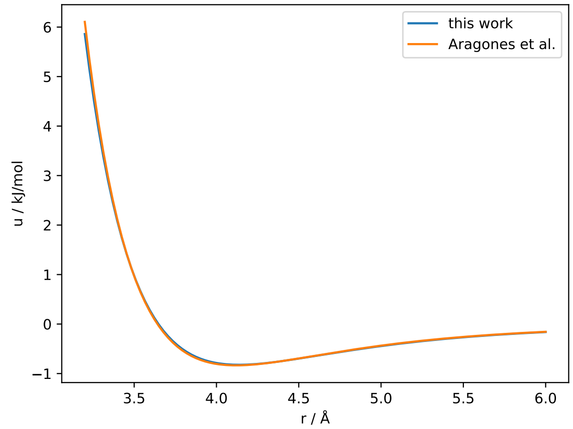


Figure 1. Cl–Cl interaction (without the Coulomb part) employed in this study and in earlier work.

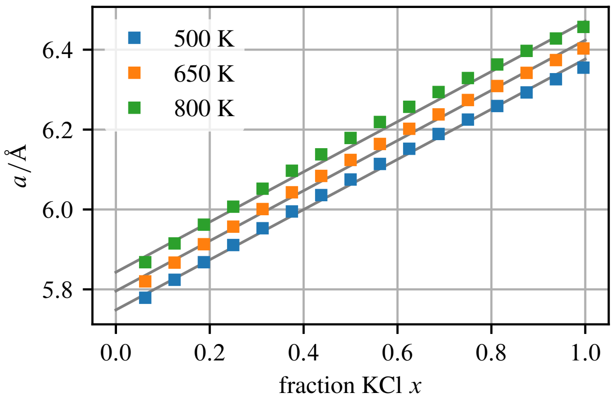


Figure 2. Lattice constant of the mixture for three selected temperatures. The thin grey lines are one common fit with a linear function of composition and temperature inspired by Vegard's law.

The parameter values are $c_x = 0.62796$ Å, $c_T = 3.1485 \times 10^{-4}$ Å/K, and $a_0 = 5.5911$ Å. Results for three different temperatures are presented in Fig. 2.

## IV. CORRELATION TEST

When using the semi-grand canonical Widom method, care has to be taken to ensure one is actually sampling a homogeneous system. In particular, there should not be any significant correlations between particle types in both time as well as position. We have a time series of system snapshots, where $t$ is used to indicate time and $i$ is labeling lattice sites. We first introduce an indicator function:

$$c_i(t) = \begin{cases} 0 & \text{site } i \text{ is occupied with Na at time } t, \\ 1 & \text{site } i \text{ is occupied with K at time } t. \end{cases} \quad (7)$$

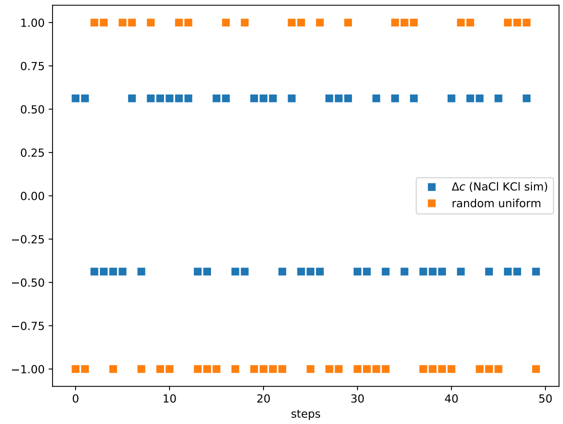


Figure 3. (Blue) $\Delta c$ as a function of steps in a time series from a real NaCl–KCl simulation, where $N_{\mathrm{K}} = 112$ and $T = 650$ K. (Orange) A series of random numbers selected with equal probability from $\{-1, 1\}$.

In the present study, all the changes happen for the Na and K atoms, while the Cl atoms always stay the same, so it is not necessary to include Cl in the indicator function. The average of this indicator function is the system composition,

$$x = \langle c_i(t) \rangle \, . \quad (8)$$

In the case of a uniform system, this average can be performed over either all lattice positions in a single configuration (fixing $t$) or all times in a time series (fixing $i$), and the result will always be the same. Next, in order to calculate a correlation function, we define

$$\Delta c_i(t) = c_i(t) - \langle c_i(t) \rangle \quad (9)$$
$$= c_i(t) - x \, . \quad (10)$$

In Fig. 3, we show $\Delta c$ for a randomly selected lattice site as a function of (arbitrary) simulation time. For comparison, we also plot a series of random numbers, which visually looks indistinguishable from the simulation data.

We now introduce a (temporal) correlation,

$$C(t) = \frac{\langle \Delta c_i(t_0) \Delta c_i(t_0 + t) \rangle}{\langle (\Delta c)^2 \rangle} , \quad (11)$$

where $\left\langle (\Delta c)^2 \right\rangle = \left\langle c^2 \right\rangle - x^2$. In the same way, we introduce a spatial correlation,

$$C_k = \frac{\langle \Delta c_i(t) \Delta c_{i+k}(t) \rangle}{\langle (\Delta c)^2 \rangle} . \quad (12)$$

Here, it is implicitely assumed that the index $i + k$ labels a particle that is $k$ crystal planes apart from the reference particle $i$. Furthermore, we assume the separation is along one of the three main directions of the crystal, and we do not count any planes containing Cl atoms. In other words, for a separation of $k = 1$, there is exactly one Cl atom between the two

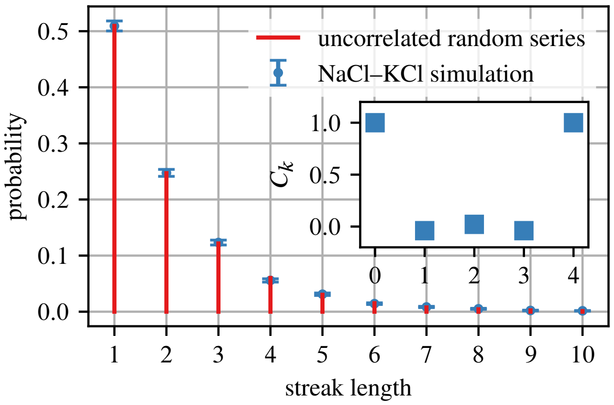


Figure 4. Distribution of streak length for one of our simulations, and for comparison the same for a Bernoulli process of same probability. (Inset) Spatial correlation function as defined in Eq. (12). For the largest separation, the correlation is 1 since due to the periodicity of the system, this is actually the reference position again.

correlated lattice positions. In the actual implementation in software, care has to be taken to correctly map between lattice indices (which correspond to specific positions in space) and standard array indices (which just number the particles from 0 to $N-1$, regardless of position).

It turns out that for our simulations and selected time interval between sampling, there is no correlation in either position or time. A spatial correlation function is shown in the inset of Fig. 4.

An alternative way of looking at correlations in time is to analyze the distribution of streak length in the corresponding time series. In our case, there are only two possible values for $\Delta c$, and the overal probability of seeing either one follows exactly from the (fixed) system composition, $x$. Consequently, if the time series is truly random, it should behave just like a Bernoulli process with $p = x$.

In such a process, each element is independent from any other, and its value is 1 with probability $p$ and 0 with probability $1 - p$. A streak of length $n$ is defined as an unbroken series of $n$ occurences of 0 or 1, terminated on both ends with the other number. In Fig. 4, we show the distribution of streak length for both a number of time series calculated from the actual simulation as well as a Bernoulli process with equal probability, which agree perfectly. If there were any correlations, these would skew the distribution of streak length with respect to he Bernoulli process.

## REFERENCES


[1] J. Anwar, D. Frenkel, and M. G. Noro, Journal of Chemical Physics **118**, 728 (2003).

[2] J. L. Aragones, E. Sanz, and C. Vega, Journal of Chemical Physics **136**, 244508 (2012).
